# Supplementary material for: In-Network View Synthesis for Interactive Multiview Video Systems
Source: arXiv:1509.00464 source file (2015-09-01)
Supplement: Supplementary file 1 [file appendix_A.tex]

{Proof of \bf\emph{Lemma 2:}} 
The scenario considered in Lemma 2 is depicted in Fig. 
\ref{fig:Lemma2}. Without loss of generality we consider the case of   $v_1=U_L$ and $v_C=U_R$. In the spirit of the DP method, we consider the case of having   $\{v_1, \ldots,  v_i\}$ as selected reference views, and we have   more views  (larger than  $v_i$) to select. As next candidate  $v_{i+1}$, we could select a synthesized view $v_n$ or a camera view $v_k$ with  $v_i< v_n <v_k <U_R$.  We can also observe that the region $[U_L,v_i]$ will be synthesized using the reference views   $\{v_1, \ldots, v_i\}$ so the selection of $v_{i+1}$ affects only the region $[v_i,U_R=v_C]$.

Equipped with these preliminary information, we can show that the regions of interest  $[v_i,v_C]$  is better reconstructed considering $v_k$ as reference view rather than $v_n$ if the conditions of the Lemma 2 holds. We discretize the region $[v_i,v_C]$ into three  sub-regions $R_1=[v_i,v_n], R_2=[v_n,v_k], $ and $R_3=[v_k,v_C]$. We now show that in each of these sub-regions, having $v_k$ as reference rather than $v_n$ leads to a lower distortion. 
\begin{align}
& d_u(v_i,\hat{v}_n^r) > d_u(v_i,v_k)  & \forall u\in R_1 \\
& d_u(\hat{v}_n^l,v_C) > d_u(v_i,v_k)  & \forall u\in R_2 \\
& d_u(\hat{v}_n^l,v_C) > d_u(v_k,v_C)  & \forall u\in R_3 
\end{align}
where in any of the above inequality  we have used the ``monotonicity in reference view distance" and the ``distorted reference view equivalence". The lhs represents the distortion of a given viewpoint $u$ when $v_i, v_n, v_C$ are available as reference views, while the rhs represents the distortion of a given viewpoint $u$ when $v_i, v_k, v_C$ are available as reference views. This shows that selecting $v_k$ is preferable over synthesizing  $v_n$.

\

\begin{figure}[t]
\begin{center}
\includegraphics[width=0.65\linewidth ,draft=false]{figure/Lemma3.eps} 
\caption{Scenario considered in Lemma 3.}
\label{fig:Lemma3}  
\end{center}
\end{figure}

{Proof of \bf\emph{Lemma 3:}} 
 If $\hat{v}_n^r \geq v_C$, proof is similar to the one of Lemma 2.  We now prove that Lemma 3 holds also if $\hat{v}_n^r < v_C$.  As before we consider three sub-regions $R_1=[v_i,v_k], R_2=[v_k,v_n], $ and $R_3=[v_n,v_C]$ and we also use the following distance notation: $N= (v_k-v_i),  L=v_n - v_k, K = v_C-\hat{v}_n^l$, and we recall that $\Delta$ is the shift of the equivalent view.   
We can easily show that 
\begin{align}
& d_u(v_i,\hat{v}_n^r) > d_u(v_i,v_k)  & \forall u\in R_1 \\
& d_u(\hat{v}_n^l,v_C) > d_u(v_k,v_C)  & \forall u\in R_3 
\end{align}
which means that both $R_1$ and $R_3$ are better reconstructed from $v_k$ than $v_n$. We now look at $R_2$
$$
\sum_{u\in R_2} d_u(v_i,\hat{v}_n^r) \ ? \ \sum_{u\in R_2}d_u(v_k,v_C)   
$$
We note that $|u-v_k| = w$ and $|u-V_r|=L-w+\Delta+K$, with $w=u-v_k$. For  $w=L, (u=v_n)$, we have 
\begin{align}\label{eq:ineq}
|u-v_k|_{u=v_n} = L < L+K< \Delta+K =  |u-v_C|_{u=v_n} 
\end{align}
where we recall that $\Delta>L $ since $\hat{v}^l_n = v_n -\Delta = v_k+L -\Delta < v_k$. Eq. \eqref{eq:ineq} states that $|u-v_k|<|u-v_C| , \ \forall uÊ\in R_2$ since it holds also for $u=v_n$ which is the  view in $R_2$ closest to $V_r$.
Finally we have $|u-v_i| = N+w, $ and $|u-\hat{v}_n^r| = L-w+\Delta$. Because of the  ``monotonicity in minimum reference view distance" we have 
\begin{align}
d_u(v_i,\hat{v}_n^r) > d_u(v_k,v_C)   \ \ \forall u\in R_2
\end{align}
if $\min\{|u-v_i|,|u-\hat{v}_n^r|\} >\min\{|u-v_k|,|u-V_r|\}$. Since
$\min\{|u-v_k|,|u-V_r|\} =|u-v_k| = w$ we have 
$$
\min\{N+w,L-w+\Delta\} > w
$$
which holds for any $u\in R_2$. This can be easily shown. If $\min\{N+w,L-w+\Delta\}= N+w$, then $N+w > w, \forall w\geq 0$ and  $\min\{N+w,L-w+\Delta\}= L-w+\Delta$, then $L-w+\Delta>w, \forall w\in[0,L]$, since even for $w=L$ we have  $\Delta> L$, which is one of the starting condition of the Lemma. 

 So also in the sub-region $R_2$, $v_k$ is preferred over $v_n$.
