# Supplementary material for: In-Network View Synthesis for Interactive Multiview Video Systems
Source: arXiv:1509.00464 source file (2015-09-01)
Supplement: Supplementary file 2 [file appendix_B.tex]

We show here why the distortion assumption   \eqref{eq:shared_optimality} and \eqref{eq:indep_optimality} hold in practice.  We first introduce   the notion of views \emph{dissimilarity}  similarly to \cite{Maug:Arxiv14,Toni:J14}. When reference view $V$  is used to synthesize a virtual viewpoint $u$,   $V$ is projected  (translated in the case of rectified cameras) into the position of $u$. During camera translation,  some background pixels   can  become hidden by foreground objects (occluded  pixels ) or  a new part of the scene may appear  in the camera because of the translation (appearing pixels).  The portion of pixels that   cannot be reconstructed from $V$ (i.e.,    occluded or appeared pixels) is what we denote by \emph{dissimilarity} among the two views. These pixels have to be recovered by inpainting techniques.    The bigger the \emph{dissimilarity}, the larger this inpainted portion, thus the greater the distortion of the synthesized viewpoint.

\subsection*{Shared optimality of references for virtual viewpoints} 
  To show the conditions under which the assumption of hared optimality of references for virtual viewpoints holds, we first consider the case in which reference views are all camera views (i.e., at the same distortion). Then we introduce the case in which reference views can be synthesized viewpoints (with a distortion proportional to the dissimilarity value).  

  Let all reference views be camera views.    For most of the 3D scenes,  the views dissimilarity increases with the  distance between the viewpoint and the reference views, and so does the distortion. This is given by the fact that,   foreground objects move faster than the background ones, resulting in occlusions or disillusion effects. Also, the  further a reference view is from a target view,
the greater the translation step from the reference view to the viewpoint, and so the greater will be the portion of appearing pixels in the scene.   So,  common 3D sequences experience  a monotonic behavior of the views dissimilarity (and so of the distortion) with the reference views distance. For scenes with this monotonic behavior with the distance, the shared optimality holds. In particular, a viewpoint $u$ is better synthesized from the pair $(V_L, V_R)$ than from $(V_L^{\prime},V_R^{\prime})$, with $V_L^{\prime}<V_L \leq u \leq V_R < V_R^{\prime}$. However, because of the monotonic behavior, also $u^{\prime}$ is better reconstructed by the pair $(V_L, V_R)$ if  $V_L \leq u^{\prime} \leq V_R$. This means the shared optimality holds.

 We are then interested in understanding when the monotonic behavior of the distortion does not hold. For this to not hold, views dissimilarity has to be non-monotonic with the reference views distance.  This can be experienced  in 3D scenes with a very close background object and a highly heterogenous background. In this case,  because of the small depth of  the object, the latter moves very fast during  the translation from   reference views to viewpoint. Thus, the foreground object can appear in $V_L$ and not in $V_L^{\prime}$, as well as it can appear in $u$ and not in $u^{\prime}$. Thus, the dissmiliraity between $u^{\prime}$ and $V_L$ is much larger than the one between $u^{\prime}$ and $V_L^{\prime}$, and  because of the lack of self-similarity of the background, the inpainted region will be recovered at large distortion. Thus, viewpoint $u^{\prime}$ might be better reconstructed by far aways reference viewpoints (i.e., there is no monotonic behavior of the distortion with distance). At the same time, views dissimilarity is lower between $u$ and $V_L$ than the one between $u$ and $V_L^{\prime}$. Thus, for these 3D scenes, the shared optimality condition does not hold.   

\

\subsection*{Independence of optimality for left and right references} 

 Let assume that $V_L$ and $V_L^{\prime}$ are two possible reference views for synthesizing $u$, with $V_L^{\prime}< V_L<u$. Let also assume that $V_R>u$ is the right reference view. All reference views are camera views. If the monotonic behavior of the distortion with the distance holds, then   $V_L$ has a smaller dissimilarity with  $u$ than $V_L^{\prime}$ and thus the distortion of the  viewpoint  synthesized from $(V_L,V_R)$ cannot be worse than the distortion when $(V_L^{\prime},V_R)$ are the reference views. This is true for any $V_R>u$. In particular,   the  pixels of $u$ reconstructed from $V_R$ might  be not overlapping with the ones  projected from the left, or i  partially overlapping or completely overlapping.  In the latter case,  $V_L$ and $V_L^{\prime}$ will provide the same distortion for the synthesized viewpoint, while in the other two cases, $u$ is better reconstructed from $V_L$.  Thus, for all the three cases,   $(V_L,V_R)$ is preferred to $(V_L^{\prime},V_R)$,  the monotonic distortion behavior holds (i.e., for most of 3D scenes) then the independence of optimality for  references holds.
