# Supplementary material for: In-Network View Synthesis for Interactive Multiview Video Systems
Source: arXiv:1509.00464 source file (2015-09-01)
Supplement: Supplementary file 3 [file appendix_B_short.tex]

We show here why the distortion assumption   \eqref{eq:shared_optimality} and \eqref{eq:indep_optimality} hold in practice.  We first introduce   the notion of views \emph{dissimilarity}  similarly to \cite{Maug:Arxiv14,Toni:J14}. When reference view $V$  is used to synthesize a virtual viewpoint $u$,   $V$ is projected  (translated in the case of rectified cameras) into the position of $u$. During camera translation,  some background pixels   can  become hidden by foreground objects (occluded  pixels ) or  a new part of the scene may appear  in the camera because of the translation (appearing pixels).  The portion of pixels that   cannot be reconstructed from $V$ (i.e.,    occluded or appeared pixels) is what we denote by \emph{dissimilarity} among the two views. These pixels have to be recovered by inpainting techniques.    The bigger the \emph{dissimilarity}, the larger this inpainted portion, thus the greater the distortion of the synthesized viewpoint.

\subsection*{Discussion of the ``independence of reference optimality" assumption} 
We first assume that all reference views are camera views.
 If the distortion of the synthesized viewpoint increases according to  the reference view distance (monotonic behavior with the distance), a viewpoint $u$ is better synthesized from the pair $(V_L, V_R)$ than from $(V_L^{\prime},V_R^{\prime})$, with $V_L^{\prime}<V_L \leq u \leq V_R < V_R^{\prime}$. Because of the monotonic behavior, this also holds for any other viewpoint $u^{\prime}\in [V_L,V_R]$. It means that the shared optimality holds if the distortion of the synthesis has a monotonic behavior with the distance between the synthetic view and the reference ones. Conventional 3D scenes  have  foreground objects that are not in the proximity of cameras. In this case, the greater the translation step from the reference view to the viewpoint (i.e., the greater the reference view distance),  the greater   the portion of appearing pixels in the scene, so the greater the dissimilarity among views.   This means that  common 3D sequences experience  a monotonic behavior of the views dissimilarity (and so of the distortion) with the reference views distance.    
 When 3D scenes have  foreground objects very close to cameras and a highly heterogenous background,  foreground objects move  very fast during  the translation from the reference views to synthetic view. This might lead to anomalous behaviors. Foreground objects can appear in $V_L$  and $u^{\prime}$ but not  in $V_L^{\prime}$ and    $u$, with $V_L^{\prime}<V_L<u<u^{\prime}$. The projection of $V_L^{\prime}$ to $u$ would have many disoccluded pixels in this case. Because of the lack of self-similarity of the background, the inpainted region will be recovered with  large distortion. This means that the dissimilarity between $u$ and $V_L$ is much larger than the one between $u$ and $V_L^{\prime}$. Thus, the viewpoint $u$ might be better reconstructed by    reference viewpoints  that are far away (i.e., there is no monotonic behavior of the distortion with distance).   
 \begin{figure}[t]
 \begin{center}
 \includegraphics[width=0.5\linewidth ,draft=false]{figure/Camera_Translation.eps} 
 \caption{Translation geometry for synthesized reference views.}\label{fig:Camera_Translation}
 \end{center}
 \end{figure}
 
  We now consider the case in which reference views are synthesized and so that they can have   different distortion values. If $V_L$ and $V_L^{\prime}$ are such that $D(V_L)\leq D(V_L^{\prime})$, with $V_L^{\prime} < V_L < u$ and common 3D scenes are considered such that the dissimilarities are monotonic with the distance,  $V_L$ is preferred since it will recover a larger portion of $u$ and at a better distortion. In this case, the distortion is monotonic with the distance and the assumption of shared optimality holds.  
Consider now the opposite case in which   $D(V_L^{\prime}) \leq D(V_L)$ and we consider common 3D scenes (monotonic dissimilarity behavior with distance) with high-quality depth maps (i.e., the synthesized reference view $V_L$ does not introduce substantial propagation errors in the depth). 
We depict an example in Fig. \ref{fig:Camera_Translation} for the sake of clarity. In the example, $V_L$ is synthesized by cameras pair $(V_a,V_b)$.  Because of the errors introduced in the inpainting process (white area in $V_L$  in Fig. \ref{fig:Camera_Translation}),  $D(V_L^{\prime})$ might be larger than the distortion of the camera view $V_L^{\prime}$. However, when we look at the synthesized viewpoint $u$, it is interesting to observe that this   distortion gap does not necessarily reflect   in   $u$. In particular, comparing the contribution that $V_L^{\prime}$ could offer to $u$ with the one offered by $V_L$, we notice that the latter has lower dissimilarity and so it offers a larger distortion. Moreover, the only area that was inpainted in $V_L$ (i.e., the only area at low-quality) would still be inpainted in $u$ if recovered from $V_L^{\prime}$. Thus,   $(V_L,V_R)$ is still preferred to $(V_L^{\prime},V_R)$. This shows that in common 3D scenes, a monotonic behavior of the distortion with the reference   distance is experienced and the shared optimality assumption holds.  

For the monotonicity of the distortion not to hold, again a particular scene has to be experienced. Namely, a very close foreground object and heterogenous background have to characterize the scene. 
Note that these are the same condition (i.e., the same specific scenes) for the assumption   not to hold in the case of only  camera views as reference views.   For these scenes, if $V_L^{\prime}< V_a <V_L<V_b<u$,  $V_L$ can an inpainted region which is out-of-view in $u$ and in $V_L^{\prime}$ as well.   In this specific configuration, $u$ is better reconstructed from $(V_L^{\prime},V_R)$ than  $(V_L,V_R)$, the monotonicity of the distortion does not  hold and neither the shared optimality assumption.  

\

To better explain the above motivation we provide the following illustrative examples.  Let consider the synthetic scene of  Fig. \ref{fig:Synthetic_example_SHARED_hold} that describes a common multiview scenario with one   foreground objects  in the scene  (labeled A in the figure) and a quite uniform background (labeled B in the figure). We consider two possible viewpoints $u$ and $u^{\prime}$,     with $V_L^{\prime}<V_L \leq u^{\prime} < u \leq V_R < V_R^{\prime}$. The views $V_L$ and $V_L^{\prime}$ are candidate left reference views while $V_R$ and $V_R^{\prime}$ are the candidate right reference views.  For each candidate reference view, we highlight the regions that contribute to the virtual synthesis of the viewpoint of interest. In particular,  dashed borders delimit the area that is projected onto the virtual view.  We notice that for   the pair $(V_L,V_R)$ reconstruct a larger portion of $u$ compared to any other combination of reference view pairs. \footnote{This is visible by the dashed border areas that are larger in  $V_L$ and $V_R$. } Because of the scene geometry,  the same observation holds   for any other $u^{\prime}$ in the range $[V_L,V_R]$. This is because in this scene with a conventional 3D geometry the the distortion of the synthesis has a monotonic behavior with the reference distance. Thus the shared optimality condition holds.  

 %%%%%%%%%
 \begin{figure} 
 \begin{center}
 \subfigure[3D scene.]{
\includegraphics[width=0.3\linewidth ,draft=false]{figure/Synthetic_example_SHARED_hold_2A.eps} }
  \subfigure[Scene captured by each view.]{
\includegraphics[width=0.9\linewidth ,draft=false]{figure/Synthetic_example_SHARED_hold_2B.eps} }
 \caption{Example in which the assumption of shared optimality of references  \emph{holds}. Areas filled with same color represent portion of the frame at the same depth. Dashed bordered areas in reference views represents the contribution from the reference to the virtual viewpoint. }\label{fig:Synthetic_example_SHARED_hold}
 \end{center}
 \end{figure}

 \begin{figure} 
  \begin{center}
 \subfigure[3D scene.]{
 \includegraphics[width=0.3\linewidth ,draft=false]{figure/Synthetic_example_SHARED_2A.eps} 
 }
 \subfigure[Scene capture by each view. Viewpoint to synthesize $u$.]{
 \includegraphics[width=0.9\linewidth ,draft=false]{figure/Synthetic_example_SHARED_2B.eps} 
 }
 \subfigure[Scene capture by each view. Viewpoint to synthesize $u^{\prime}$.]{
 \includegraphics[width=0.9\linewidth ,draft=false]{figure/Synthetic_example_SHARED_2C.eps} 
 } \caption{Example in which the assumption of shared optimality of references \emph{does not hold}. Areas filled with same color represent portion of the frame at the same depth. Dashed bordered areas in reference views represents the contribution from the reference to the virtual viewpoint. }\label{fig:Synthetic_example_SHARED}
 \end{center}
 \end{figure}

For the shared optimality condition  not to     hold, we need to consider a specific 3D scene where   the foreground object   is very close to one or more camera views and the background is  highly heterogenous. This creates an irregular (non monotonic) behavior of the occlusions experienced with the distance. An example is provided in  Fig.  \ref{fig:Synthetic_example_SHARED}, where the foreground object   is very close to the camera $V_R$. Because of its vicinity   to the camera, the foreground object  appears in camera view $V_R$ as well as in viewpoint $u$, but not in camera view $V_R^{\prime}$ nor in viewpoint $u^{\prime}$. This creates an irregular behavior on the areas that can be reconstructed in $u^{\prime}$. For example, camera view $V_R$ is closer to $u^{\prime}$ than $V_R^{\prime}$, but it   offers a contribution only in the reconstruction of region B in $u^{\prime}$, while 
$V_R^{\prime}$ allows to reconstruct both regions B and D.  Thus, $(V_L, V_R^{\prime})$ is the best reference views pair for $u^{\prime}$. However, this does not hold for $u$, where region A can only be reconstructed from reference view $V_R$ and not $V_R^{\prime}$. Thus, for synthesizing viewpoint $u$ the best reference views pair is $(V_L, V_R)$. This contradicts the shared optimality condition. 
 %%%%%%%%%

%  \begin{figure}[t]
% \begin{center}
% \includegraphics[width=0.5\linewidth ,draft=false]{figure/Camera_Translation.eps} 
% \caption{Translation geometry for synthesized reference views.}\label{fig:Camera_Translation}
% \end{center}
% \end{figure}

We now consider the case in which a non uniform distortion is experienced within one reference frame. For example, if a reference view is a synthesized one, some areas can be reconstructed by impainting, leading to a higher distortion than the non-occluded ones. In this case, for the shared optimality assumption to do not hold, we still have to be in a very peculiar case. For example, a viewpoint $u$ might have a region of interest A which can be reconstructed from $V_R$ at low distortion and from $V_R^{\prime}$ at high distortion. Thus, the former is preferred as right reference view for $u$. If  $u^{\prime}$ is such that this region is no more in the scene of $u^{\prime}$ \emph{and} the contribution of $V_R^{\prime}$ is better than the one offered from $V_R$, $V_R^{\prime}$ is preferred as right view for $u^{\prime}$. This could be possible only if the high-distortion region in $V_R^{\prime}$ was delimited to the region of interest A and not to the other ones \emph{and} the  remaining region cannot be provided at low-distortion from $V_R$.

\subsection*{Discussion of the ``independence of reference optimality" assumption} 
 Let assume that $V_L$ and $V_L^{\prime}$ are two possible reference views for synthesizing $u$, with $V_L^{\prime}< V_L<u$. Let also assume that $V_R>u$ is the right reference view. All reference views are camera views. If the monotonic behavior of the distortion with the distance holds, then   $V_L$ has a smaller dissimilarity with  $u$ than $V_L^{\prime}$ and thus the distortion of the  viewpoint  synthesized from $(V_L,V_R)$ cannot be worse than the distortion when $(V_L^{\prime},V_R)$ are the reference views. This is true for any $V_R>u$. %In particular,   the  pixels of $u$ reconstructed from $V_R$ might  be not overlapping with the ones  projected from the left, or i  partially overlapping or completely overlapping.  In the latter case,  $V_L$ and $V_L^{\prime}$ will provide the same distortion for the synthesized viewpoint, while in the other two cases, $u$ is better reconstructed from $V_L$.  Thus, for all the three cases,   $(V_L,V_R)$ is preferred to $(V_L^{\prime},V_R)$,  
 Thus, when the monotonic distortion behavior holds (i.e., for most of 3D scenes), the independence of optimality for  references holds.

 We now consider a specific 3D scene such that the monotonic distortion behavior is not guaranteed. Moreover, the scene is such that non-occluded pixels in $u$ when reconstructed from $V_L$  are complementary to the  pixels  reconstructed from $V_R$ and almost identical to the  non-occluded pixels in $u$ when reconstructed from $V_R^{\prime}$. In this very specific case, the  independence of optimality for  references does not hold. Similar considerations can be derived from the case in which reference views do not have the same distortion. For the assumption  not to hold the 3D scene has to be  a very specific one. With the same reasoning of the  shared optimality condition, it can be shown that these specific scenes are also the one in which  the independence optimality does not holds when reference views are synthesized.  
 
 \
 
%We first consider the case in which reference views have the same distortion or has a uniform allocation of the rate within the frame (i.e., there is no a region with much higher distortion than others). Similarly to the above assumption, in scenes with monotonic behavior with distance, the independence of optimality holds. Considering the example in Fig. \ref{fig:Synthetic_example_SHARED_hold}, the viewpoint $u$ is better reconstructed from $V_R$ rather than $V_R^{\prime}$, no matter which left view is selected. Same for the left views. 

   \begin{figure}[t]
 \begin{center}
  \subfigure[3D scene.]{
 \includegraphics[width=0.3\linewidth ,draft=false]{figure/Synthetic_example_INDEP_2A.eps} 
 }
  \subfigure[Scene capture by each view. ]{
 \includegraphics[width=0.9\linewidth ,draft=false]{figure/Synthetic_example_INDEP_2B.eps} 
 }
 \caption{Example in which the assumption of independence of optimality of references views  \emph{does not hold}. Areas filled with same color represent portion of the frame at the same depth. Dashed bordered areas in reference views represents the contribution from the reference to the virtual viewpoint. }\label{fig:Synthetic_example_INDEP}
 \end{center}
 \end{figure}
 
 We now provide an example to better understand the  independence of optimality for  references. 
For the assumption to do not hold, we need to be in a peculiar scenario in which one right reference  view  is complementary to a given  left reference  view and not to another left reference view. To better understand this scenario, we consider Fig. \ref{fig:Synthetic_example_INDEP}, where three foreground objects and a uniform background is considered. However, two  foreground objects (orange cylinders) are very close to camera views, while the third one (red ball) is more far away. The scene at the viewpoint $u$ is given by the red foreground object (region A) and a background (region B), but not from the two cylinders. However, shifting the perspective of the scene on the right or on the left introduces an obstacle in both views $V_R$ and $V_L$. This obstacles are close enough to the cameras to be not present anymore in $V_R^{\prime}$ and $V_L^{\prime}$. This results in a scenario in which the contribution offered from $V_R$ for $u$ is complementary to the one offered from $V_L$, while it is redundant w.r.t. to the one offered from $V_L^{\prime}$. Also the contribution offered from $V_R^{\prime}$ is complementary to the one given by $V_L^{\prime}$ and similar to the one from $V_L$. This means that the $V_R$ is the best right reference view if $V_L$ is the selected left reference view, otherwise (if $V_L^{\prime}$ is the left reference view) $V_R^{\prime}$ is preferred. Thus, the assumption of independence of optimality does not hold. 

Analogously, in case of non uniform distortion across the acquired frame, for the assumption to do not hold we would need to be in a specific scenario in which the regions of high distortion offered from a right reference views are complementary to the one of high distortion from a right view and similar to the one of another right reference view.

\

Thus, we have shown that in the most common 3D scenes both assumptions hold. For them to not be respected we need to capture   very specific 3D scenes.
