# Supplementary material for: In-Network View Synthesis for Interactive Multiview Video Systems
Source: arXiv:1509.00464 source file (2015-09-01)
Supplement: Supplementary file 4 [file appendix_D.tex]

From the graphical representation of reference selections in Section~\ref{subsec:graphical}, we see that, without loss of generality, a solution to \eqref{eq:optimization} can be expressed as a set of consecutive ranges or \textit{segments} of virtual views, $\theta_1, \theta_2, \ldots$, where all virtual views $u$ in a given segment $\theta_i$, $u \in \theta_i = [u_i, u_{i+1})$, share the same left and right reference views $v_L(i)$ and $v_R(i)$, respectively, and $v_L(i) \leq u_i < u_{i+1} - \frac{1}{L} \leq v_R(i)$. Further, adopting the shared reference optimality assumption, any two neighboring segments in an optimal solution, $\theta^*_i = [u_i, u_{i+1})$ and $\theta^*_{i+1} = [u_{i+1}, u_{i+2})$, must satisfy the following condition: either the right reference $v_R(i)$ of segment $\theta^*_i$ is also the right boundary $u_{i+1} - \frac{1}{L}$ of $\theta^*_i$, or the left reference $v_L(i+1)$ of segment $\theta^*_{i+1}$ is also the left boundary $u_{i+1}$ of $\theta^*_{i+1}$. Failure to meet both of the above conditions would mean boundary virtual views $u_{i+1} - \frac{1}{L}$ and $u_{i+1}$ can both use $(v_L(i), v_R(i))$ and $(v_L(i+1), v_R(i+1))$ as references, and given segments $\theta^*_i$ and $\theta^*_{i+1}$ assign them different reference pairs, the solution cannot be optimal.

Given the above observation, we can construct an optimal algorithm by constructing one segment $\theta_i$ at a time. We first define $\Phi(u, \Theta, k)$ as the minimum aggregate synthesized view distortion from virtual view $u$ to $U^0_R$, given segments in set $\Theta$ have selected left references but not right references, and $k$ additional reference views can be selected.

\begin{equation}
\Phi(u, v_L, \Theta, k) = 
\min_{\substack{v \in \mathcal{V} | v > u \\ \Theta' \subseteq \Theta \cup \theta_k}} \left\{
\Phi(v + \frac{1}{L}, \Theta \cup \theta_k \setminus \Theta', k-1) + 
\sum_{\theta_i \in \Theta'} \sum_{u \in [u_i, u_{i+1})} 
d_u(v_L(i), v, D(v_L(i)), D(v))
\right\}
\end{equation}
where new segment $\theta_k = [u, v)$ with

Let consider the $i$-th optimization step ($i>1$), in which the first $C-k$ reference views has been already selected, and the remaining $k$ has to be discovered.  At this step, $v_i>v_{i-1}$ has to be optimized, where $v_{i-1}$ is the reference views selected at the $(i-1)$-th optimization step. 
We denote by $\mathcal{L}: \{v_1, v_2, \ldots, v_{|\mathcal{L}|}\}$ the set of   reference views selected up to the current step. This means that $v_{|\mathcal{L}|}= v_{i-1}$ at the $i$-th step. Also, since we impose $v_i>v_{i-1}$ at each optimization step, we have   $v_1 < v_2 < \ldots < v_{|\mathcal{L}|}$. 
Each selected reference view $v_l$  greater than $U_L^0$ forms a viewpoint range $[ \max\{U_L^0, v_{l-1}\}, \min\{U_R^0, v_{l}\}]$
that shares the same reference views (for the shared optimality of references for virtual viewpoints). In general, we denote by $\theta:  [U_L(\theta), U_R(\theta)]$ the resulting viewpoint range characterized by the most left and right viewpoints, denoted by $U_L(\theta)$  and $U_R(\theta)$, respectively.  At the $i$-th optimization step, we denote by $\Psi:\{\theta_1, \theta_2, \ldots \}$ the set of viewpoint ranges $\theta$ that are still looking for the best reference views  pair to be used for the range. 

We are then interested in finding the best $v_i$ using the following recursion
\begin{align}\label{eq:optimal_alternat_1}
\Phi(\mathcal{L}, \Psi, k) &= \min_{v_i > v_{|\mathcal{L}|}} \left\{ \Phi(\mathcal{L} \cup v_i, \Psi \cup  \theta^{\prime}\setminus \Omega, k-1) + \sum_{\theta \in \Omega}  \min_{\substack{V_L\leq u: \\  V_L \in \mathcal{L}}}
\left\{\sum_{u=U_L(\theta)}^{U_R(\theta)}  d_u^s(V_L,v_i ,d(V_L),d(v_i)) \right \}    \right\}
\end{align}
where $ \theta^{\prime} = [\max\{U_R^0, v_{|\mathcal{L}|}\}, \min\{ v_i, U_L^0\} ]$ is the new viewpoint range that $v_i$ generated and 
$\Omega \subseteq  \{\Psi \cup  \theta^{\prime}\}$ is the set of ranges that do not have the best reference views pair in $\mathcal{L}$ but they have it in  $\mathcal{L}\cup v_i$. This means that $\Omega$ is the set of ranges that have $v_i$  as best right reference view. Note that we do not associate a priori the best left reference view for each set but we optimally evaluate it in Eq. \eqref{eq:optimal_alternat_1} since in this case we do not assume   the independence of optimality for left and right references assumption.  

If none of the ranges in $ \{\Psi \cup  \theta^{\prime}\}$ have the best reference views pair in $\mathcal{L} \cup v_i$, then $\Omega = \emptyset$, while if all ranges have the best reference views pair in $\mathcal{L} \cup v_i$, then $\Omega = \Psi \cup  \theta^{\prime}$. 

In  Eq. \eqref{eq:optimal_alternat_1}  we have that 
\begin{align}\label{eq:optimal_alternat_2}
\Phi(\mathcal{L}, \Psi, 1) &= \min_{v_i > v_{|\mathcal{L}|}} \left\{  \sum_{\theta \in \{ \mathcal{L} \cup v_i\} }  \min_{\substack{V_L\leq u: \\  V_L \in \mathcal{L}}}
\left\{\sum_{u=U_L(\theta)}^{U_R(\theta)}  d_u^s(V_L,v_i ,d(V_L),d(v_i)) \right \}    \right\}
\end{align}
and 
$$
\Phi(\emptyset ,\emptyset, C)  =   {D}(\mathcal{T}^{\star},U_L^0, U_R^0)
$$
