# Supplementary material for: In-Network View Synthesis for Interactive Multiview Video Systems
Source: arXiv:1509.00464 source file (2015-09-01)
Supplement: Supplementary file 6 [file Appendix_B_old.tex]

We now   analyze both the shared optimality of references for virtual viewpoints  and the independence of optimality for left and right references assumptions for the distortion of virtual viewpoints and we show that in the most common scenarios these assumptions hold.  {Before this, we introduce the notion of views \emph{dissimilarity}. Let consider a reference view $V$  that is used to synthesize a virtual viewpoint $u$. This means that the view $V$ is projected  (translated in the case of rectified cameras) into the position of $u$. During camera translation,  some background pixels     become hidden by foreground objects (occlusion) or some background pixels in $u$ can appear behind foreground objects (disocclusion). Moreover,   a new part of the scene may appear  in the camera because of the translation.  The portion of pixels that   cannot be reconstructed from $V$ (i.e.,  either occluded or appeared pixels) is what we denote by \emph{dissimilarity} among the two views. These pixels have to be recovered by inpainting techniques.    The bigger the \emph{dissimilarity}, the larger this inpainted portion, thus the greater the distortion of the synthesized viewpoint. } 
 

\subsection*{Shared optimality of references for virtual viewpoints} 
  To show the conditions under which the assumption of hared optimality of references for virtual viewpoints holds, we first consider the case in which reference views are all camera views (i.e., at the same distortion). Then we introduce the case in which reference views can be synthesized viewpoints (with a distortion proportional to the dissimilarity value).  

  Let all reference views be camera views.    For most of the 3D scenes,  the views dissimilarity increases with the  distance between the viewpoint and the reference views, and so does the distortion. This is given by the fact that,   foreground objects move faster than the background ones, resulting in occlusions or disillusion effects. Also, the  further a reference view is from a target view,
the greater the translation step from the reference view to the viewpoint, and so the greater will be the portion of appearing pixels in the scene.   So,  common 3D sequences experience  a monotonic behavior of the views dissimilarity (and so of the distortion) with the reference views distance. For scenes with this monotonic behavior with the distance, the shared optimality holds. In particular, a viewpoint $u$ is better synthesized from the pair $(V_L, V_R)$ than from $(V_L^{\prime},V_R^{\prime})$, with $V_L^{\prime}<V_L \leq u \leq V_R < V_R^{\prime}$. However, because of the monotonic behavior, also $u^{\prime}$ is better reconstructed by the pair $(V_L, V_R)$ if  $V_L \leq u^{\prime} \leq V_R$. This means the shared optimality holds. 


 We are then interested in understanding when the monotonic behavior of the distortion does not hold. For this to not hold, views dissimilarity has to be non-monotonic with the reference views distance.  This can be experienced  in 3D scenes with a very close background object and a highly heterogenous background. In this case,  because of the small depth of  the object, the latter moves very fast during  the translation from   reference views to viewpoint. Thus, the foreground object can appear in $V_L$ and not in $V_L^{\prime}$, as well as it can appear in $u$ and not in $u^{\prime}$. Thus, the dissmiliraity between $u^{\prime}$ and $V_L$ is much larger than the one between $u^{\prime}$ and $V_L^{\prime}$, and  because of the lack of self-similarity of the background, the inpainted region will be recovered at large distortion. Thus, viewpoint $u^{\prime}$ might be better reconstructed by far aways reference viewpoints (i.e., there is no monotonic behavior of the distortion with distance). At the same time, views dissimilarity is lower between $u$ and $V_L$ than the one between $u$ and $V_L^{\prime}$. Thus, for these 3D scenes, the shared optimality condition does not hold.   

\

  \begin{figure}[t]
 \begin{center}
 \includegraphics[width=0.5\linewidth ,draft=false]{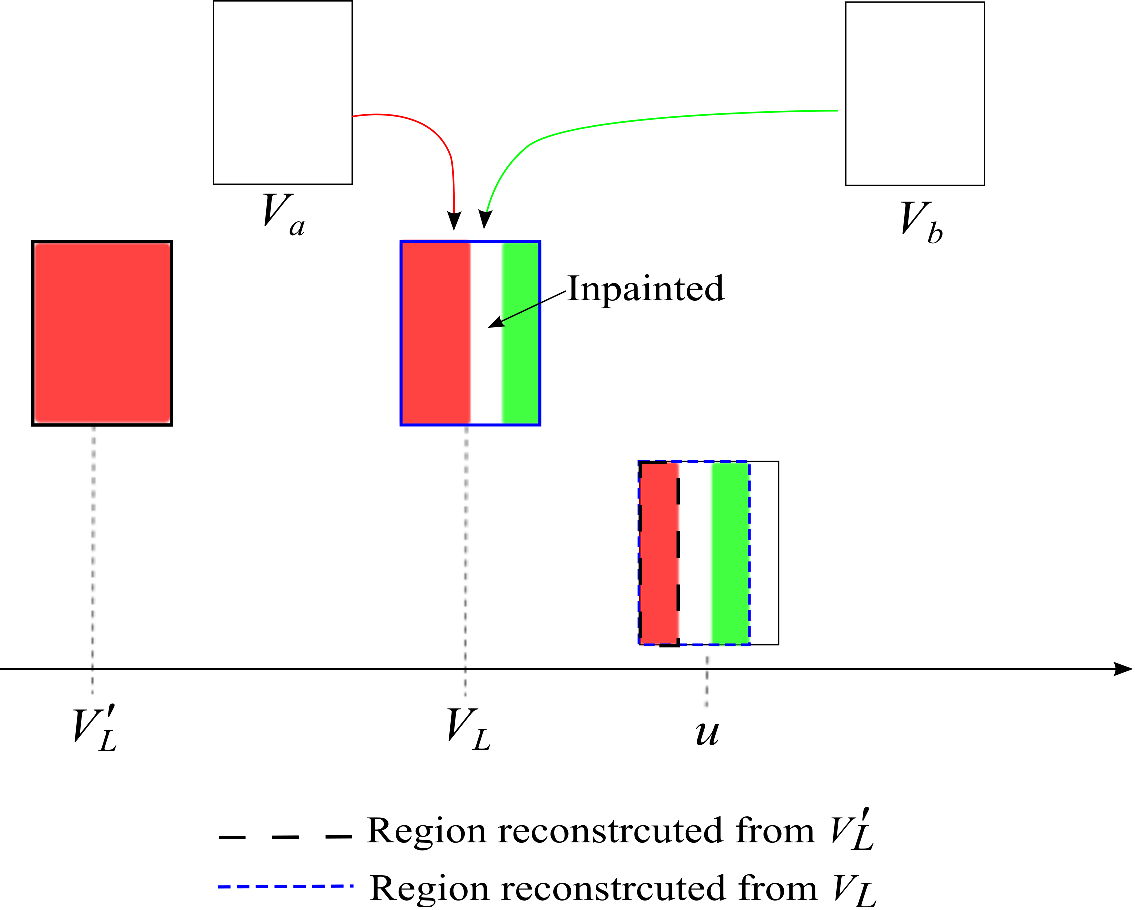} 
 \caption{Translation geometry for synthesized reference views.}\label{fig:Camera_Translation}
 \end{center}
 \end{figure}
 
 


 We now consider the case in which reference views are synthesized. This translates in having reference views with different distortion values. Let first consider the case in which $V_L^{\prime}$ is synthesized while $V_L$ is a camera view, with $V_L^{\prime}< V_L$ and also $D(V_L)\leq D(V_L^{\prime})$.  In a common 3D scene in which the dissimilarities are monotonic with the distance,  $V_L$ has less dissimilarity with $u$ than $V_L^{\prime}$. Thus, $V_L$ is preferred since it will recovere a larger portion of $u$ and at a better distortion. So, distortion is monotonic with distance and shared optimality holds.  
Let now consider the opposite case in which $V_L^{\prime}$ is a camera view  while $V_L$ is a synthesized viewpoint, leading to  $D(V_L^{\prime})\leq D(V_L)$. We depict an example in Fig. \ref{fig:Camera_Translation} for the sake of clarity. In the example, $V_L$ is synthesized by cameras pair $(V_a,V_b)$. We consider common 3D scenes (monotonic dissimilarity behavior with distance) and   ideal depth maps (i.e., the synthesized reference view $V_L$ does not introduce propagation errors in the depth). We also observe that  $D(V_L^{\prime})$ might be larger than a camera view distortion because of the errors introduced in the inpainting process (white area in $V_L$  in Fig. \ref{fig:Camera_Translation}). However, when we look at the synthesized viewpoint $u$, it is interesting to observe that this increased distortion does not necessarily reflect into an increased distortion in   $u$. In particular, comparing the contribution that $V_L^{\prime}$ could offer to $u$ with the one offered by $V_L$, we notice that the latter has lower dissimilarity and so it offers a larger contribution. Moreover, the only area that was inpainted in $V_L$ (i.e., the only area at low-quality) would still be inpainted in $u$ if recovered from $V_L^{\prime}$. Thus,   $(V_L,V_R)$ is still preferred to $(V_L^{\prime},V_R)$. This shows that in common 3D scenes, a monotonic behavior of the distortion with distance is experienced and the shared optimality assumption holds.  

 
For the monotonicity of the distortion not to hold, again a particular scene has to be experienced. Namely, a very close foreground object and heterogenous background have to characterize the scene. 
Note that these are the same condition (i.e., the same specific scenes) for the assumption   not to hold in the case of only  camera views as reference views.   For these scenes, if $V_L^{\prime}< V_a <V_L<V_b<u$,  $V_L$ can an inpainted region which is out-of-view in $u$ and in $V_L^{\prime}$ as well.   In this specific configuration, $u$ is better reconstructed from $(V_L^{\prime},V_R)$ than  $(V_L,V_R)$, the monotonicity of the distortion does not  hold and neither the shared optimality assumption.  

\begin{figure}[t]
 \begin{center}
 \subfigure[3D scene.]{
\includegraphics[width=0.3\linewidth ,draft=false]{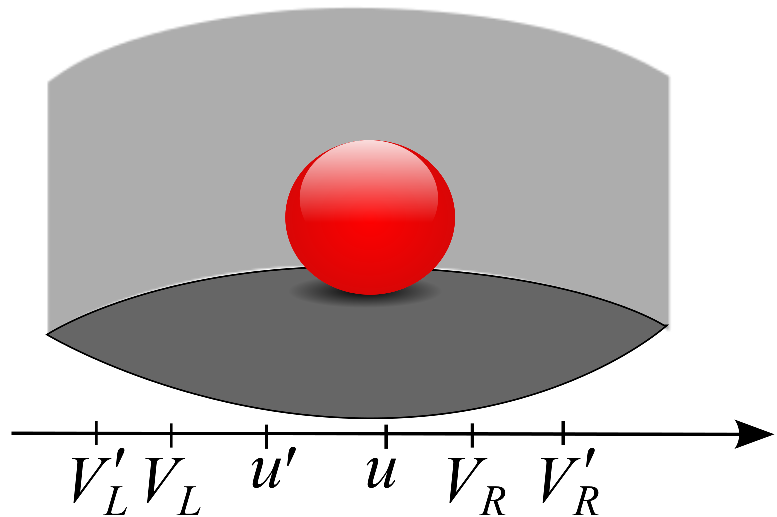} }
  \subfigure[Scene captured by each view.]{
\includegraphics[width=0.9\linewidth ,draft=false]{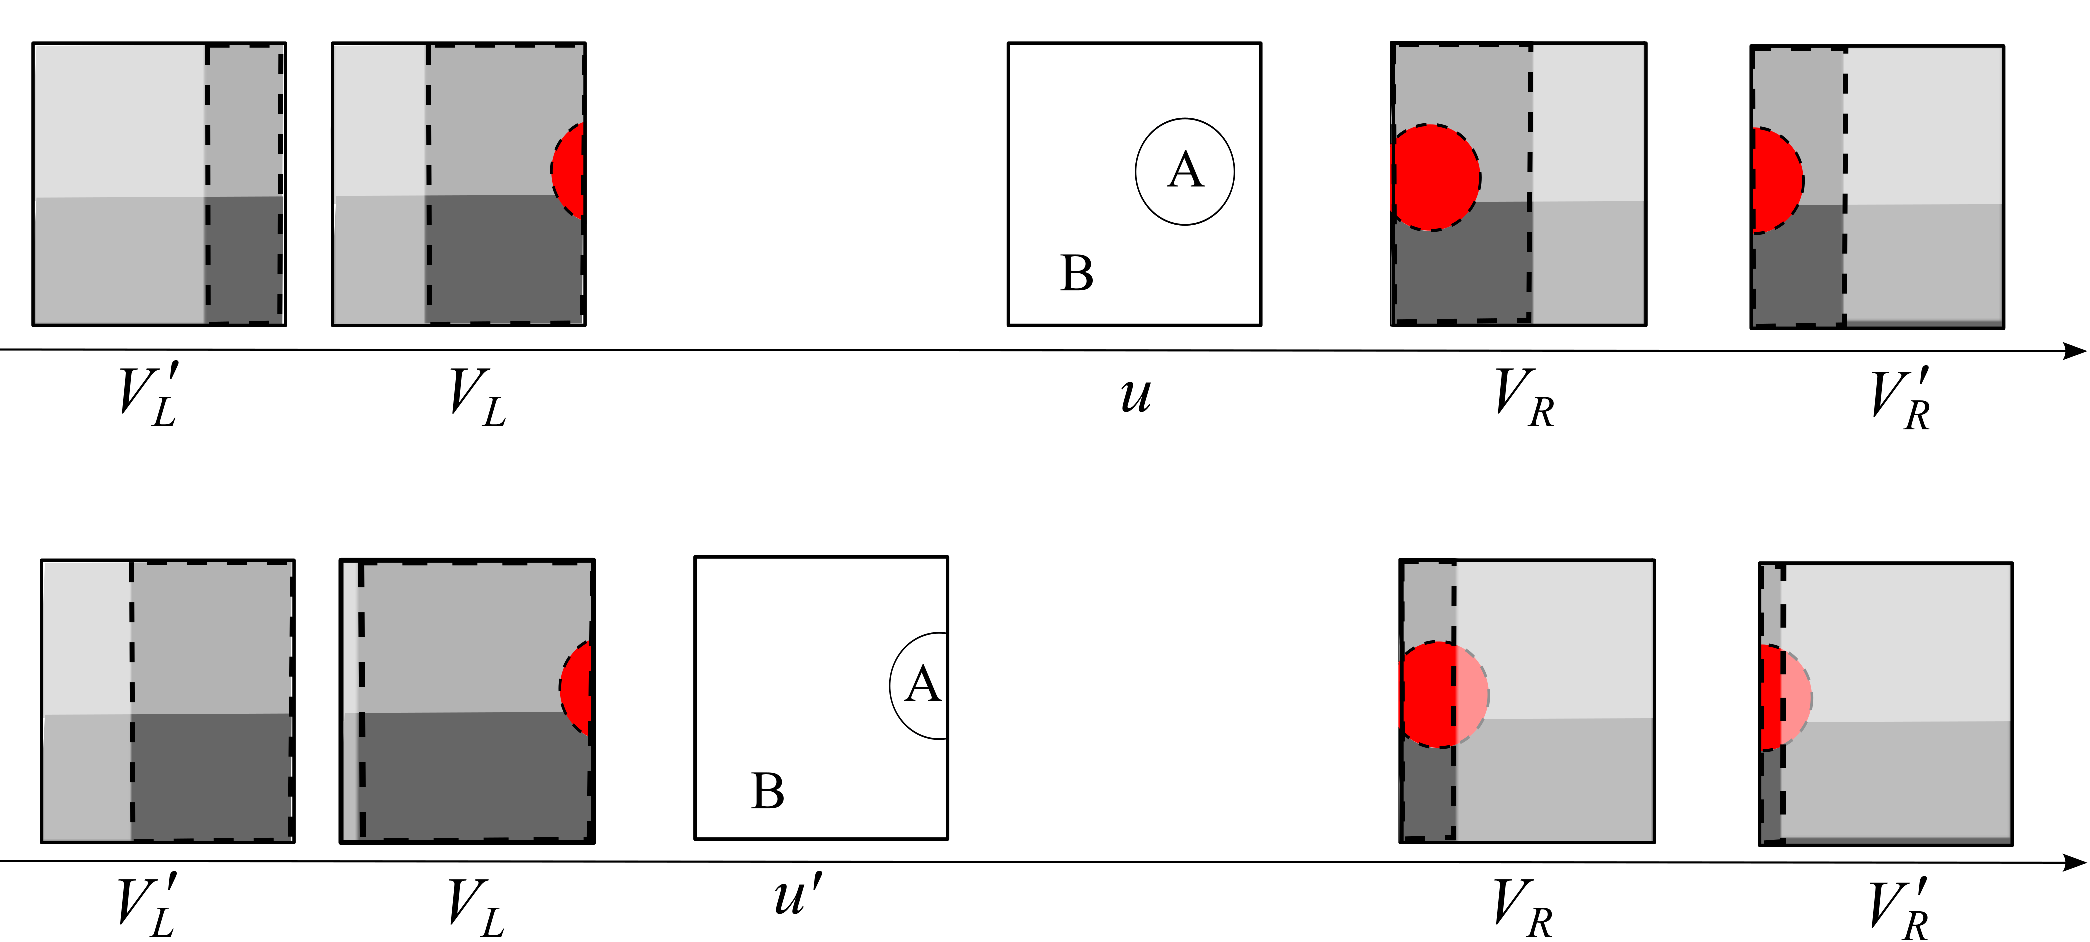} }
 \caption{Example in which the assumption of shared optimality of references  \emph{holds}. Areas filled with same color represent portion of the frame at the same depth. Dashed bordered areas in reference views represents the contribution from the reference to the virtual viewpoint. }\label{fig:Synthetic_example_SHARED_hold}
 \end{center}
 \end{figure}
 
We now show few examples to better explain the above motivation.   
We now consider the synthetic scene of  Fig. \ref{fig:Synthetic_example_SHARED_hold}, that  provides an example of reconstruction of virtual viewpoints $u$ and $u^{\prime}$ and we assume reference views to have the same distortion. For the synthesis of both viewpoints, either $V_L$ or $V_L^{\prime}$ is selected as right reference view, and one between $V_L$ and $V_L^{\prime}$ is the best left view. In each viewpoint ($u, u^{\prime}$), the frame is subdivided into regions which are reconstructed from different reference views.  For each frame acquired by a camera view, we highlight the regions that contribute to the virtual synthesis of the viewpoint of interest. In particular,    shade borders delimit the area that will be projected onto the virtual view.  

The synthetic scene  in Fig.  \ref{fig:Synthetic_example_SHARED_hold}   describes a common multiview scenario with one or more foreground objects in the scene and a quite uniform background. This scene has a monotonic behavior of the reconstructed area with the distance. This means that the larger is the distance between $u$ and the reference views, the lower is the contribution that  a reference view can offer to $u$.   In this   scenario, it can then be observed that the shared optimality condition holds.  In particular, the assumption  states that if  $(V_L,V_R)$ is preferred to $(V_L^{\prime},V_R)$ as reference views pair for the viewpoint $u$, then it will be preferred also for $u^{\prime}$, with  $\min{v_L, v_L^{\prime}} \leq u, u^{\prime} \leq v_R$. This is the case in scenarios like the one in Fig. \ref{fig:Synthetic_example_SHARED_hold}. 

 \begin{figure}[t]
 \begin{center}
 \subfigure[3D scene.]{
 \includegraphics[width=0.3\linewidth ,draft=false]{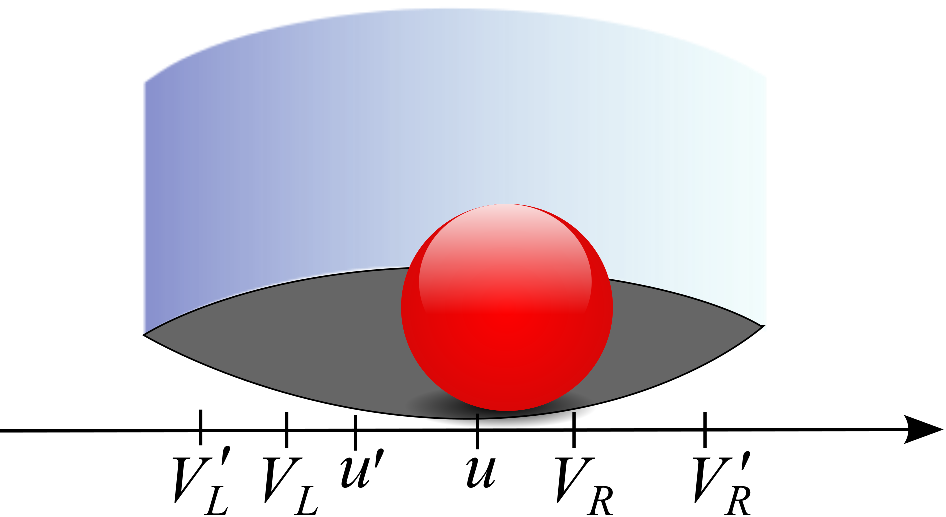} 
 }
 \subfigure[Scene capture by each view. Viewpoint to synthesize $u$.]{
 \includegraphics[width=0.9\linewidth ,draft=false]{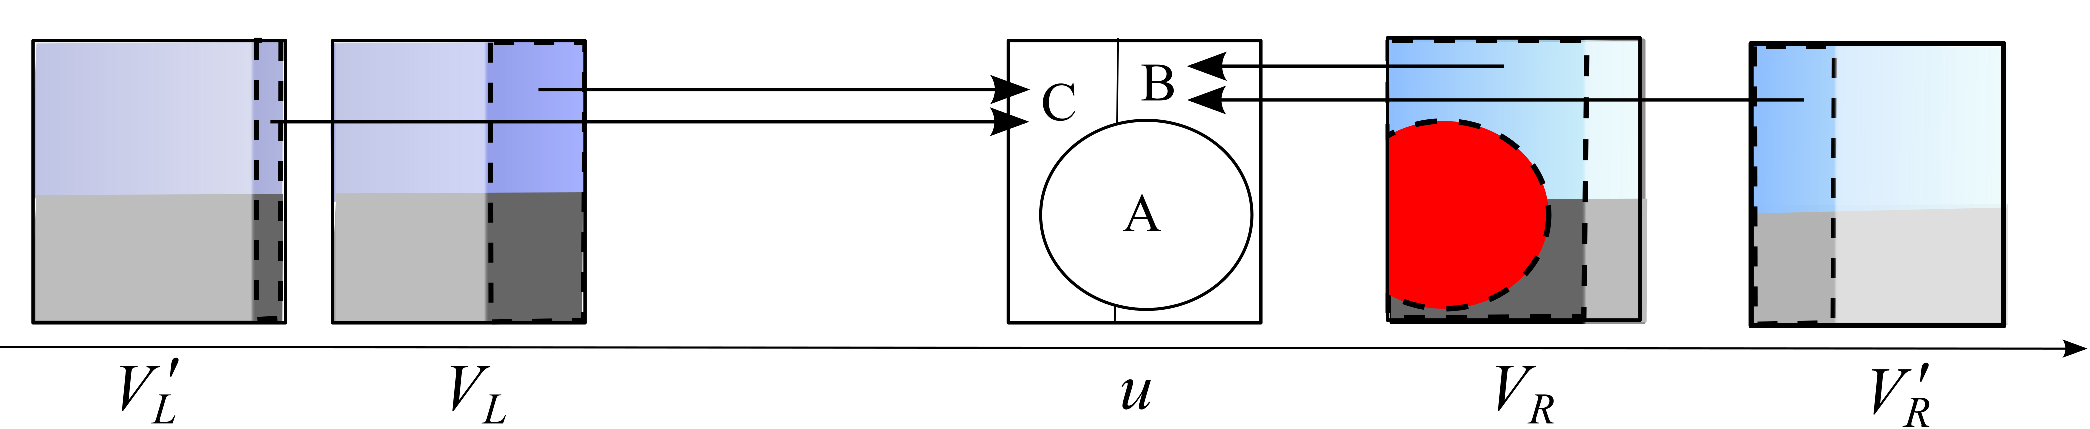} 
 }
 \subfigure[Scene capture by each view. Viewpoint to synthesize $u^{\prime}$.]{
 \includegraphics[width=0.9\linewidth ,draft=false]{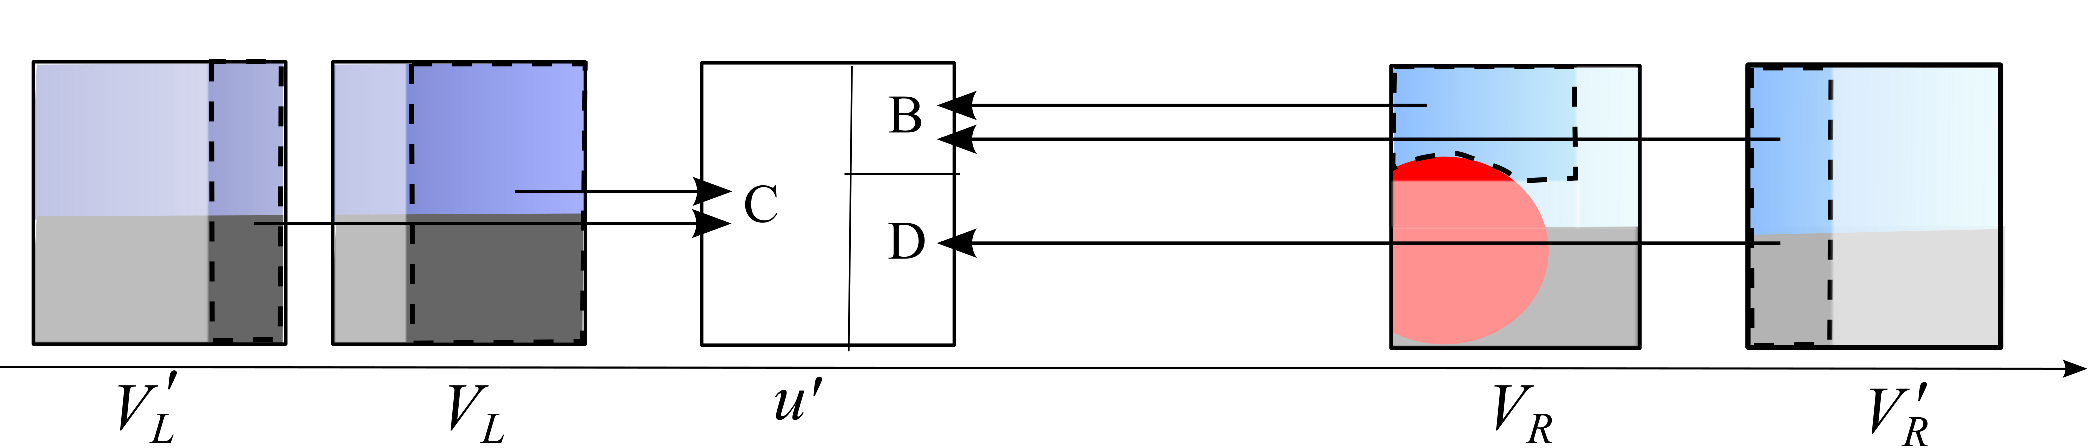} 
 } \caption{Example in which the assumption of shared optimality of references \emph{does not hold}. Areas filled with same color represent portion of the frame at the same depth. Dashed bordered areas in reference views represents the contribution from the reference to the virtual viewpoint. }\label{fig:Synthetic_example_SHARED}
 \end{center}
 \end{figure}

For the shared optimality condition to do not hold, we need to consider a specific 3D scene where some camera views have a foreground object which is very close to one or more camera view and the background is   heterogenous. This creates an irregular (non monotonic) behavior of the occlusions experienced with the distance. An example is provided in  Fig.  \ref{fig:Synthetic_example_SHARED}, where the foreground object   very close to the camera $V_R$. Because of its vicinity   to the camera, the foreground object  appears in camera view $V_R$ as well as in viewpoint $u$, but not in camera view $V_R^{\prime}$ nor in viewpoint $u^{\prime}$. This creates an irregular behavior on the areas that can be reconstructed in $u^{\prime}$. For example, camera view $V_R$ is closer to $u^{\prime}$ than $V_R^{\prime}$, but it   offers a contribution only in the reconstruction of region B in $u^{\prime}$, while 
$V_R^{\prime}$ allows to reconstruct both regions B and D.  Thus, $(V_L, V_R^{\prime})$ is the best reference views pair for $u^{\prime}$. However, this does not hold for $u$, where region A can only be reconstructed from reference view $V_R$ and not $V_R^{\prime}$. Thus, for synthesizing viewpoint $u$ the best reference views pair is $(V_L, V_R)$. This contradicts the shared optimality condition. 


We now consider the case in which a non uniform distortion is experienced within one reference frame. For example, if a reference view is a synthesized one, some areas can be reconstructed by impainting, leading to a higher distortion than the non-occluded ones. In this case, for the shared optimality assumption to do not hold, we still have to be in a very peculiar case. For example, a viewpoint $u$ might have a region of interest A which can be reconstructed from $V_R$ at low distortion and from $V_R^{\prime}$ at high distortion. Thus, the former is preferred as right reference view for $u$. If  $u^{\prime}$ is such that this region is no more in the scene of $u^{\prime}$ \emph{and} the contribution of $V_R^{\prime}$ is better than the one offered from $V_R$, $V_R^{\prime}$ is preferred as right view for $u^{\prime}$. This could be possible only if the high-distortion region in $V_R^{\prime}$ was delimited to the region of interest A and not to the other ones \emph{and} the  remaining region cannot be provided at low-distortion from $V_R$. 



 %%
\subsection*{Independence of optimality for left and right references} 

 Let assume that $V_L$ and $V_L^{\prime}$ are two possible reference views for synthesizing $u$, with $V_L^{\prime}< V_L<u$. Let also assume that $V_R>u$ is the right reference view. All reference views are camera views. If the monotonic behavior of the distortion with the distance holds, then   $V_L$ has a smaller dissimilarity with  $u$ than $V_L^{\prime}$ and thus the distortion of the  viewpoint  synthesized from $(V_L,V_R)$ cannot be worse than the distortion when $(V_L^{\prime},V_R)$ are the reference views. This is true for any $V_R>u$. In particular,   the  pixels of $u$ reconstructed from $V_R$ might  be not overlapping with the ones  projected from the left, or i  partially overlapping or completely overlapping.  In the latter case,  $V_L$ and $V_L^{\prime}$ will provide the same distortion for the synthesized viewpoint, while in the other two cases, $u$ is better reconstructed from $V_L$.  Thus, for all the three cases,   $(V_L,V_R)$ is preferred to $(V_L^{\prime},V_R)$,  the monotonic distortion behavior holds (i.e., for most of 3D scenes) then the independence of optimality for  references holds.  
 
 We now consider a specific 3D scene such that the monotonic distortion behavior is not guaranteed. Moreover, the scene is such that non-occluded pixels in $u$ when reconstructed from $V_L$  are complementary to the  pixels  reconstructed from $V_R$ and almost identical to the  non-occluded pixels in $u$ when reconstructed from $V_R^{\prime}$. In this very specific case, the  independence of optimality for  references does not hold. Similar considerations can be derived from the case in which reference views do not have the same distortion. For the assumption  not to hold the 3D scene has to be  a very specific one. With the same reasoning of the  shared optimality condition, it can be shown that these specific scenes are also the one in which  the independence optimality does not holds when reference views are synthesized.  
 
 \
 
%We first consider the case in which reference views have the same distortion or has a uniform allocation of the rate within the frame (i.e., there is no a region with much higher distortion than others). Similarly to the above assumption, in scenes with monotonic behavior with distance, the independence of optimality holds. Considering the example in Fig. \ref{fig:Synthetic_example_SHARED_hold}, the viewpoint $u$ is better reconstructed from $V_R$ rather than $V_R^{\prime}$, no matter which left view is selected. Same for the left views. 

 
   \begin{figure}[t]
 \begin{center}
  \subfigure[3D scene.]{
 \includegraphics[width=0.3\linewidth ,draft=false]{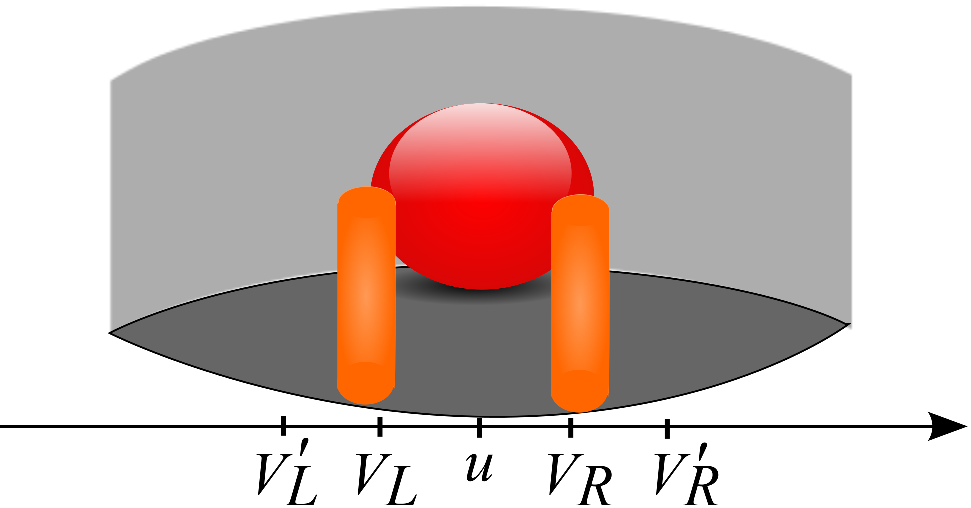} 
 }
  \subfigure[Scene capture by each view. ]{
 \includegraphics[width=0.9\linewidth ,draft=false]{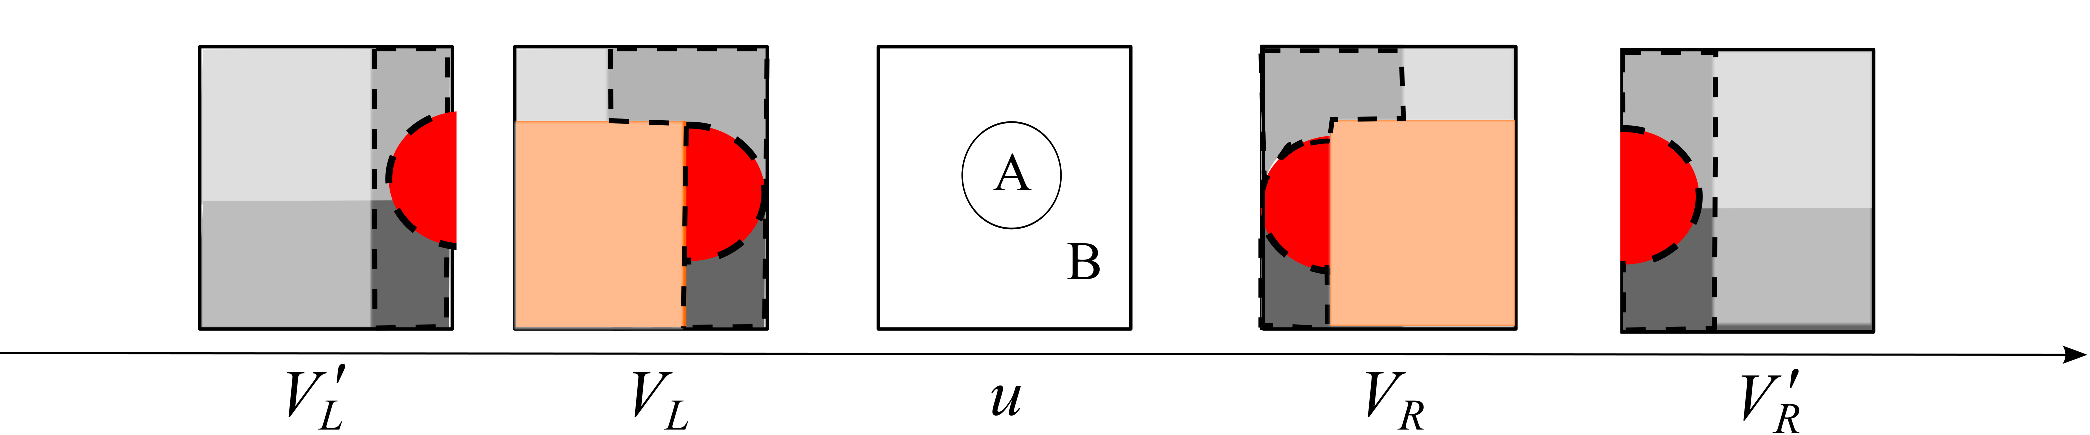} 
 }
 \caption{Example in which the assumption of independence of optimality of references views  \emph{does not hold}. Areas filled with same color represent portion of the frame at the same depth. Dashed bordered areas in reference views represents the contribution from the reference to the virtual viewpoint. }\label{fig:Synthetic_example_INDEP}
 \end{center}
 \end{figure}
 
 We now provide an example to better understand the  independence of optimality for  references. 
For the assumption to do not hold, we need to be in a peculiar scenario in which one right reference  view  is complementary to a given  left reference  view and not to another left reference view. To better understand this scenario, we consider Fig. \ref{fig:Synthetic_example_INDEP}, where three foreground objects and a uniform background is considered. However, two  foreground objects (orange cylinders) are very close to camera views, while the third one (red ball) is more far away. The scene at the viewpoint $u$ is given by the red foreground object (region A) and a background (region B), but not from the two cylinders. However, shifting the perspective of the scene on the right or on the left introduces an obstacle in both views $V_R$ and $V_L$. This obstacles are close enough to the cameras to be not present anymore in $V_R^{\prime}$ and $V_L^{\prime}$. This results in a scenario in which the contribution offered from $V_R$ for $u$ is complementary to the one offered from $V_L$, while it is redundant w.r.t. to the one offered from $V_L^{\prime}$. Also the contribution offered from $V_R^{\prime}$ is complementary to the one given by $V_L^{\prime}$ and similar to the one from $V_L$. This means that the $V_R$ is the best right reference view if $V_L$ is the selected left reference view, otherwise (if $V_L^{\prime}$ is the left reference view) $V_R^{\prime}$ is preferred. Thus, the assumption of independence of optimality does not hold. 

Analogously, in case of non uniform distortion across the acquired frame, for the assumption to do not hold we would need to be in a specific scenario in which the regions of high distortion offered from a right reference views are complementary to the one of high-distortion from a right view and similar to the one of another right reference view. 


\

Thus, we have shown that in the most common 3D scenes both assumptions hold. For them to not be respected we need to capture   very specific 3D scenes. 
